# Supplementary material for: Topics, Authors, and Institutions in Large Language Model Research: Trends from 17K arXiv Papers
Source: arXiv:2307.10700 source file (2024-04-28)
Supplement: Supplementary file 1 [file supp_table_enriched_subarxivs.tex]

\begin{table*}
\small
\centering

\caption{\textbf{Sub-arXivs that 2023 LLM authors are enriched for publishing in, excluding their LLM papers.} Sub-arXivs are sorted by how much more likely an LLM author from 2023 is to have published in that sub-arXiv compared to a publication count-matched non-LLM author. Sub-arXivs are displayed only if $\ge 2\%$ of authors, overall, have published in them; $p$-values computed with a $\chi^2$ test. We use ``sub'' as short-hand for sub-arXiv.}

\label{appendix:enriched-subarxivs-llm-auth}

\begin{tabular}{lcccc}
\toprule
                                       sub-arXiv & $\frac{p(\text{sub-arXiv} \mid \text{LLM author})}{p(\text{sub-arXiv} \mid \text{non-LLM author})}$ & $p(\text{sub} \mid \text{LLM author})$ & $p(\text{sub} \mid \text{non-LLM author})$ &  $p$-value \\
\midrule
                       Computation and Language &             5.43 &           0.52 &               0.10 &  0.0e+00 \\
                          Information Retrieval &             2.78 &           0.17 &               0.06 & 3.0e-118 \\
                                          Sound &             1.98 &           0.09 &               0.04 &  1.2e-31 \\
                           Software Engineering &             1.75 &           0.08 &               0.05 &  2.4e-21 \\
                                      Databases &             1.49 &           0.05 &               0.03 &  9.6e-08 \\
                                     Multimedia &             1.47 &           0.04 &               0.03 &  3.4e-06 \\
                        Artificial Intelligence &             1.44 &           0.21 &               0.15 &  4.6e-31 \\
                      Social and Info.~Networks &             1.40 &           0.10 &               0.07 &  1.2e-11 \\
                     Human-Computer Interaction &             1.26 &           0.09 &               0.07 &  5.5e-06 \\
                          Computers and Society &             1.24 &           0.08 &               0.06 &  4.7e-05 \\
                                Computer Vision &             1.06 &           0.46 &               0.43 &  1.8e-04 \\
                               Machine Learning &             1.02 &           0.53 &               0.52 &  1.0e-01 \\
                      Cryptography and Security &             0.98 &           0.12 &               0.13 &  5.3e-01 \\
              Neural Computing &             0.92 &           0.04 &               0.05 &  2.4e-01 \\
                          Hardware Architecture &             0.88 &           0.02 &               0.02 &  1.9e-01 \\
                                       Robotics &             0.75 &           0.11 &               0.15 &  8.0e-15 \\
                          Distributed Computing &             0.71 &           0.07 &               0.10 &  6.6e-12 \\
                                       Graphics &             0.67 &           0.02 &               0.03 &  1.9e-05 \\
                                      Stat - ML &             0.65 &           0.09 &               0.14 &  3.3e-25 \\
                             Multiagent Systems &             0.64 &           0.03 &               0.04 &  8.1e-08 \\
Comp.~Eng, Finance, and Sci &             0.62 &           0.02 &               0.03 &  4.4e-06 \\
                            Stat - Applications &             0.62 &           0.03 &               0.05 &  3.0e-11 \\
                        Networking and Internet &             0.58 &           0.05 &               0.09 &  1.6e-23 \\
                             Stat - Methodology &             0.55 &           0.04 &               0.08 &  1.7e-23 \\
                             Information Theory &             0.47 &           0.05 &               0.11 &  9.3e-50 \\
                             CS and Game Theory &             0.42 &           0.02 &               0.06 &  1.9e-28 \\
                            Systems and Control &             0.41 &           0.01 &               0.03 &  2.9e-18 \\
                    Data Structs and Algorithms &             0.37 &           0.03 &               0.07 &  1.0e-42 \\
\bottomrule
\end{tabular}
\end{table*}
